# Supplementary material for: Imaging non-collinear antiferromagnetic textures via single spin relaxometry
Source: arXiv:2006.13130 ancillary file (2020-06-23)
Supplement: Supplementary file 1 [file supplement.pdf]

# Supplementary Information

## Imaging antiferromagnetic textures via single spin relaxometry

Aurore Finco,<sup>1</sup> Angela Haykal,<sup>1</sup> Rana Tanos,<sup>1</sup> Florentin Fabre,<sup>1</sup> Saddam Chouiaeb,<sup>1</sup> Waseem Akhtar,<sup>1</sup> Isabelle Robert-Philip,<sup>1</sup> William Legrand,<sup>2</sup> Fernando Ajejas,<sup>2</sup> Karim Bouzehouane,<sup>2</sup> Nicolas Reyren,<sup>2</sup> Thibaut Devolder,<sup>3</sup> Jean-Paul Adam,<sup>3</sup> Joo-Von Kim,<sup>3</sup> Vincent Cros,<sup>2</sup> and Vincent Jacques<sup>1</sup>

<sup>1</sup>*Laboratoire Charles Coulomb, Université de Montpellier and CNRS, 34095 Montpellier, France*

<sup>2</sup>*Unité Mixte de Physique, CNRS, Thales, Université Paris-Saclay, 91767 Palaiseau, France*

<sup>3</sup>*Centre de Nanosciences et de Nanotechnologies, CNRS, Université Paris-Saclay, 91120 Palaiseau, France*

### CONTENTS

|                                                                      |    |
|----------------------------------------------------------------------|----|
| I. Magnetic characterization of the samples                          | 2  |
| II. Calculation of the PL dependence on $T_1$                        | 3  |
| III. Micromagnetics simulations                                      | 4  |
| A. Principle of the calculation of the noise maps                    | 4  |
| B. Simulated dispersion relation for spin spirals                    | 6  |
| C. Simulated noise spectrum of an isolated SAF skyrmion              | 7  |
| D. Thermal power spectral density of the SAF uniform resonance mode  | 8  |
| IV. Additional experimental data                                     | 10 |
| A. Quantitative analysis of the domain wall profile                  | 10 |
| B. Measurements of $T_1$ above non-magnetic surfaces                 | 11 |
| C. Additional relaxation time measurements on the spin spiral sample | 12 |
| D. Additional relaxation time measurements on the skyrmion sample    | 13 |
| References                                                           | 13 |

## I. MAGNETIC CHARACTERIZATION OF THE SAMPLES

The magnetic multilayers have been deposited by d.c. magnetron sputtering at room temperature on thermally oxidized silicon substrates, under Ar gas flow at a pressure of 0.25 Pa with deposition rates calibrated beforehand by x-ray reflectivity measurements. The base pressure of the sputtering equipment was  $5 \times 10^{-6}$  Pa. All multilayers described in this work have been deposited on top of Ta(5 nm)/Pt(8 nm) buffers and capped with Pt(3 nm) layers to prevent oxidation.

A preliminary characterization of the sample magnetization have been performed using an alternating gradient magnetometry setup, on  $4 \text{ mm} \times 4 \text{ mm}$  films. The out-of-plane magnetization hysteresis loops of the multilayer SAFs imaged in Figs. 2 and 5 are presented in Fig. S1. They consist of the average out-of-plane magnetization component  $m_z$  summed over all magnetic layers, which is measured as a function of the externally applied out-of-plane magnetic field  $\mu_0 H_z$ . The loop for the SAF with  $t_{\text{Co}} = 1.41 \text{ nm}$  shows a rather flat central plateau at zero magnetization ended by transitions toward saturated magnetization states at its two ends, indicative of a significant effective magnetic anisotropy (Fig. S1a). The SAF with  $t_{\text{Co}} = 1.47 \text{ nm}$  rather shows a linear evolution of its average  $m_z$  towards saturation (Fig. S1b), here characteristic of a vanishing effective anisotropy allowing for the stabilization of a spin-spiral state under zero external field. For the biased SAF, this loop is superimposed to the one of the bias layer, which appears in Fig. S1c as the central rectangular sharp loop. The remaining of the curve features the evolution of  $m_z$  in the SAF system coupled to it, with the same linear evolution, as  $t_{\text{Co}} = 1.47 \text{ nm}$ . These curves also reveal that the SAF system hosts a compensated magnetic configuration at zero external field, in all three cases. The magnetic anisotropy of the films has been deduced from in-plane magnetization measurements using the method of areas [1].

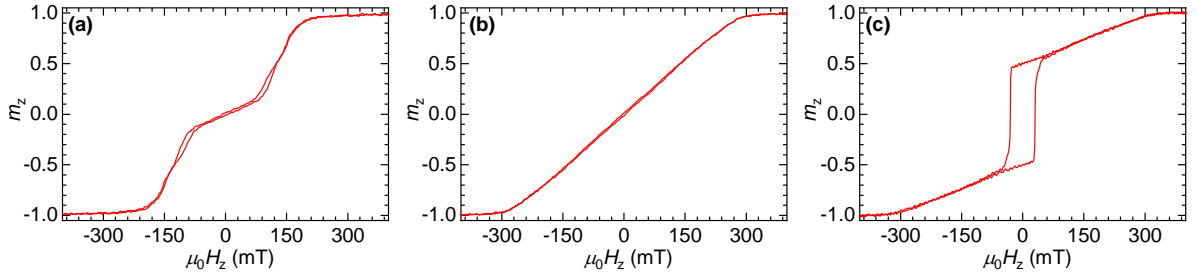

FIG. S1. **Hysteresis loops.** Average out-of-plane magnetization component  $m_z$  of the full stacks for **a**, the domain wall sample ( $t_{\text{Co}} = 1.41 \text{ nm}$ ), **b**, the spiral sample ( $t_{\text{Co}} = 1.47 \text{ nm}$ ) and **c**, the skyrmion sample ( $t_{\text{Co}} = 1.47 \text{ nm}$  with an additional bias layer).

## II. CALCULATION OF THE PL DEPENDENCE ON $T_1$

We consider the simple two-level system presented in Fig. 1a to infer the evolution of the NV defect PL signal with  $T_1$ . Under continuous optical illumination with a power  $P$ , the steady state spin populations ( $n_0^{\text{st}}, n_1^{\text{st}}$ ) result from the competition between the longitudinal spin relaxation rate  $\Gamma_1 = 1/2T_1$ , and optically-induced spin polarization in the  $m_s = 0$  spin sublevel with a rate  $\Gamma_p$ , which can be expressed as

$$\Gamma_p = \Gamma_p^\infty \frac{P}{P + P_{\text{sat}}} ,$$

where  $P_{\text{sat}}$  denotes the saturation power of the optical transition and  $\Gamma_p^\infty \simeq 5 \times 10^6 \text{ s}^{-1}$  is the polarization rate at saturation [2].

The PL rate  $\mathcal{R}$  of the NV defect can be written as

$$\mathcal{R} = \frac{P}{P + P_{\text{sat}}} (\alpha n_0^{\text{st}} + \beta n_1^{\text{st}}) \quad (1)$$

where  $\alpha$  and  $\beta$  are phenomenologically introduced to take into account that the  $m_s = 0$  spin sublevel is brighter than  $m_s = \pm 1$  ( $\alpha > \beta$ ) [2]. Using this simple model, the steady state spin populations are given by

$$n_0^{\text{st}} = \frac{\Gamma_1 + \Gamma_p}{2\Gamma_1 + \Gamma_p} , \quad n_0^{\text{st}} + n_1^{\text{st}} = 1 \quad (2)$$

which leads to

$$\mathcal{R} = \frac{P}{P + P_{\text{sat}}} \frac{\alpha(\Gamma_1 + \Gamma_p) + \beta\Gamma_1}{2\Gamma_1 + \Gamma_p} . \quad (3)$$

The curves shown in Fig. 1a are calculated for two different optical excitation power while using  $\alpha = 1$  and  $\beta = 0.6$ .

### III. MICROMAGNETICS SIMULATIONS

The magnetic noise spectrum is investigated using numerical micromagnetics with the MUMAX3 code [3, 4]. The SAF structure was modelled as a rectangular trilayer system with dimensions of  $L_x \text{ nm} \times L_y \text{ nm} \times 4.5 \text{ nm}$  that is discretised with  $N_x \times N_y \times 3$  finite difference cells. According to experimental measurements on the samples, we use a saturation magnetization of  $M_s = 1.2 \text{ MA m}^{-1}$ , a ferromagnetic intralayer exchange of  $A = 20 \text{ pJ m}^{-1}$ , and a uniaxial magnetic anisotropy along the  $z$  axis, perpendicular to the film plane. For the domain wall system, we consider a uniaxial anisotropy constant of  $K_u = 0.945 \text{ MJ m}^{-3}$ , an interfacial Dzyaloshinskii-Moriya constant of  $D = 0.9 \text{ mJ m}^{-2}$ , and an antiferromagnetic interlayer exchange coupling of  $A_{\text{RKKY}} = -0.3 \text{ mJ m}^{-2}$ , while for spin spiral and skyrmion system we consider  $K_u = 0.895 \text{ MJ m}^{-3}$  (leading to a nearly vanishing  $K_{\text{eff}} = K_u - \mu_0 M_s^2/2$ ),  $D = 0.85 \text{ mJ m}^{-2}$ , and  $A_{\text{RKKY}} = -0.27 \text{ mJ m}^{-2}$ . For the skyrmion system, an additional bias field of  $\mu_0 H_b = 50 \text{ mT}$  is applied to the bottom layer of the SAF, which mimics an exchange bias coupling. For the domain wall system, periodic boundary conditions are applied along the  $y$  direction, parallel to the length of the domain wall, while for the spin spiral and skyrmion systems periodic boundaries are applied in both the  $x$  and  $y$  directions. A Gilbert damping constant of  $\alpha = 0.1$  was used for all systems.

The dispersion relations in Fig. 4b-c were constructed from the transient response to a time-dependent magnetic field of the form  $\mathbf{b}_{\text{rf}}(y, t) = b_0(t) [\cos(k_n y)\hat{\mathbf{x}} + \sin(k_n y)\hat{\mathbf{y}}]$  for the uniform state and  $\mathbf{b}_{\text{rf}}(y, t) = b_0(t) [\cos(k_n y)\hat{\mathbf{x}} + \sin(k_n y)\hat{\mathbf{z}}]$  for the domain wall and spin spiral, where  $b_0(t) = \sin(\pi \nu t)/\pi \nu t$  is a sinc function with  $\nu = 50 \text{ GHz}$  and amplitude of  $1 \text{ mT}$ , while  $k_n = 2\pi n/N_y$  is a quantized wave vector along the propagation direction,  $y$ . For all simulations we used  $N_y = 2048$ ,  $L_y = 10\,240 \text{ nm}$ , while  $N_x = 64$ ,  $L_x = 160 \text{ nm}$  for the uniform state,  $N_x = 256$ ,  $L_x = 640 \text{ nm}$  for the domain wall, and  $N_x = 128$ ,  $L_x = 250 \text{ nm}$  for the spin spiral configuration. For each value of the wave vector  $k_n$ ,  $b_{\text{rf}}(t)$  was applied to the system starting from the initial relaxed magnetic configuration and the damped magnetic response was simulated over  $20 \text{ ns}$ . The power spectrum was then computed from the Fourier transform of this magnetic response. Let  $l = 1, 2$  denote the top and bottom layers of the SAF, respectively. In Fig. 4, we present the dispersion relations corresponding to the sum response,  $\mathbf{m}_+ = (\mathbf{m}_1 + \mathbf{m}_2)/2$ , which represents the net magnetization that would be probed experimentally.

#### A. Principle of the calculation of the noise maps

To estimate the relevant magnetic noise spectrum for the relaxometry measurements, we computed the response of the SAF to a random spatial field which simulates thermal fluctuations, but with a harmonic time dependence at the frequency of  $f_0 = 2.87 \text{ GHz}$ . The idea is to estimate the power spectrum of magnetic fluctuations at  $f_0$  by computing the magnetic susceptibility at this frequency. This random field varies between each finite difference cell, where its orientation is drawn from a uniform distribution over the unit sphere (i.e., the  $z$  component is taken to be a random value between  $[1, -1]$  and the azimuthal angle is drawn randomly from the interval  $[0, 2\pi)$ ), while its magnitude is drawn from a Gaussian distribution centred at zero with a variance of  $1 \text{ mT}$  (see Fig. S2a). The random field is applied to a relaxed magnetic state and the simulation geometry for all cases is  $N_x = N_y = 512$ ,  $L_x = L_y = 750 \text{ nm}$ .

The noise map is computed as follows. For a given realisation  $i$  of the random magnetic

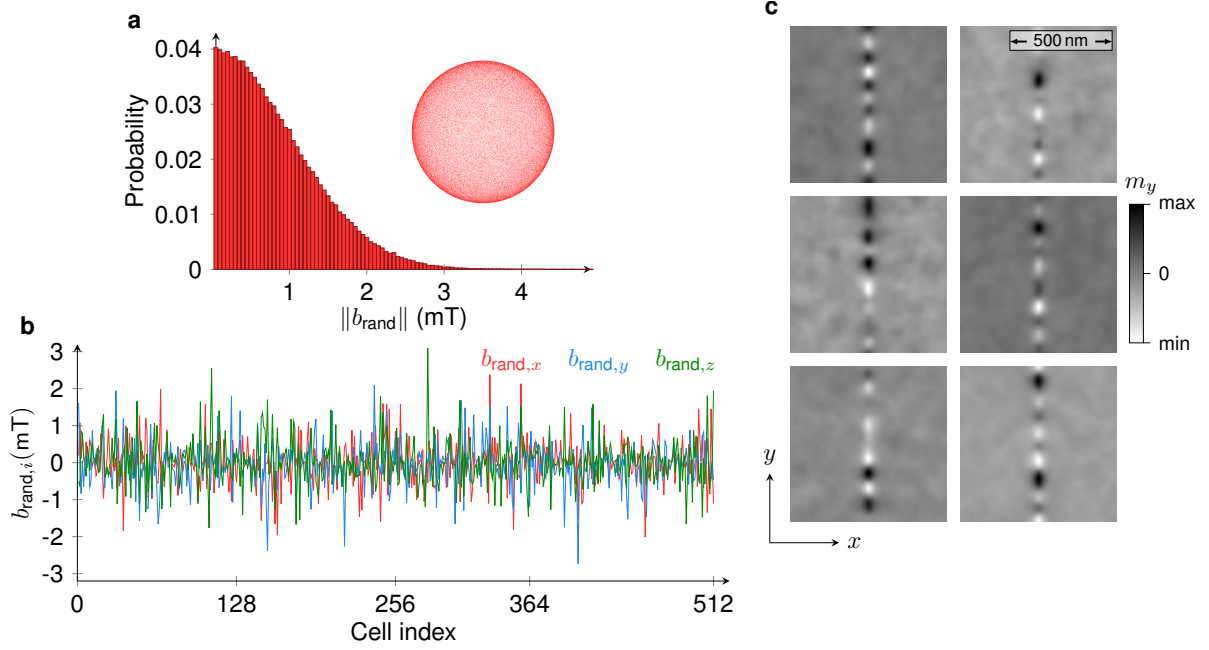

FIG. S2. **Random field excitation for noise intensity maps.** **a**, Probability distribution of field magnitude for one realisation of the spatial random field,  $\mathbf{b}_{\text{rand}}(\mathbf{r}, t)$ . The inset shows the field orientations projected onto the unit sphere. **b**, Example of a line cut of one realisation of the random field across the width of the simulation grid. **c**, Six snapshots of the  $m_y$  response in the bottom SAF layer to different realizations of the random spatial field with a sinusoidal time dependence at a frequency of 2.87 GHz.

field, the dynamics is calculated using the MUMAX3 code over one period of the 2.87 GHz excitation and the micromagnetic state is recorded. We then compute the deviation in the stray magnetic field with respect to the relaxed state  $\mathbf{m}_0$ ,  $\delta\mathbf{B}_i = \mathbf{B}_i - \mathbf{B}_0$ , at a height of 80 nm above the multilayer, which corresponds to the flying distance of the NV spin sensor. The square of the magnitude of the projection of this field along the direction perpendicular to the NV axis,  $\|\delta\mathbf{B}_{\perp,i}\|^2$ , is then recorded at each position of the simulation grid. This projection operation is motivated by the fact that the longitudinal spin relaxation time of the NV defect is only sensitive to the magnetic noise component perpendicular to the NV axis [5]. The noise maps shown in Figs. 4d, S3d,f and S4d,f represent an average of  $\|\delta\mathbf{B}_{\perp,i}\|^2$  over 500 different realizations of the random driving field.

Magnetic disorder was included to obtain more realistic static magnetization profiles, such as roughening of domain walls and spin spirals, and non axially-symmetric skyrmions. Disorder was simulated by local fluctuations in the uniaxial anisotropy constant. By using Voronoi tessellation, we divided the bilayer into a distribution of grains [4] in the film plane with an average grain size of 10 nm. The anisotropy constant in each grain  $j$ ,  $K_{u,j}$ , was drawn from a Gaussian distribution centred on the base value  $K_{u,0}$  used previously with a spread of 5%. The ground state magnetization was computed by relaxing the equilibrium profile computed in the disorder-free cases in the presence of these grains.

## B. Simulated dispersion relation for spin spirals

With the micromagnetics parameters given at the beginning of section III, we first initialize the system with a sinusoidal magnetization state with a wave vector along the  $x$  direction and the magnetic moments rotating in the  $xz$ -plane. To model the experimental system, the initial state comprises one full period over the size of the supercell of 250 nm, with periodic conditions applied along both the  $x$  and  $y$  directions. The moments in the top and bottom layers of the SAF are aligned in antiparallel with a left-handed chirality, as appropriate for the sign of the Dzyaloshinskii-Moriya interaction chosen. This initial trial state is then relaxed toward an equilibrium state by minimizing the energy. The relaxed configuration is shown in Figure S3a.

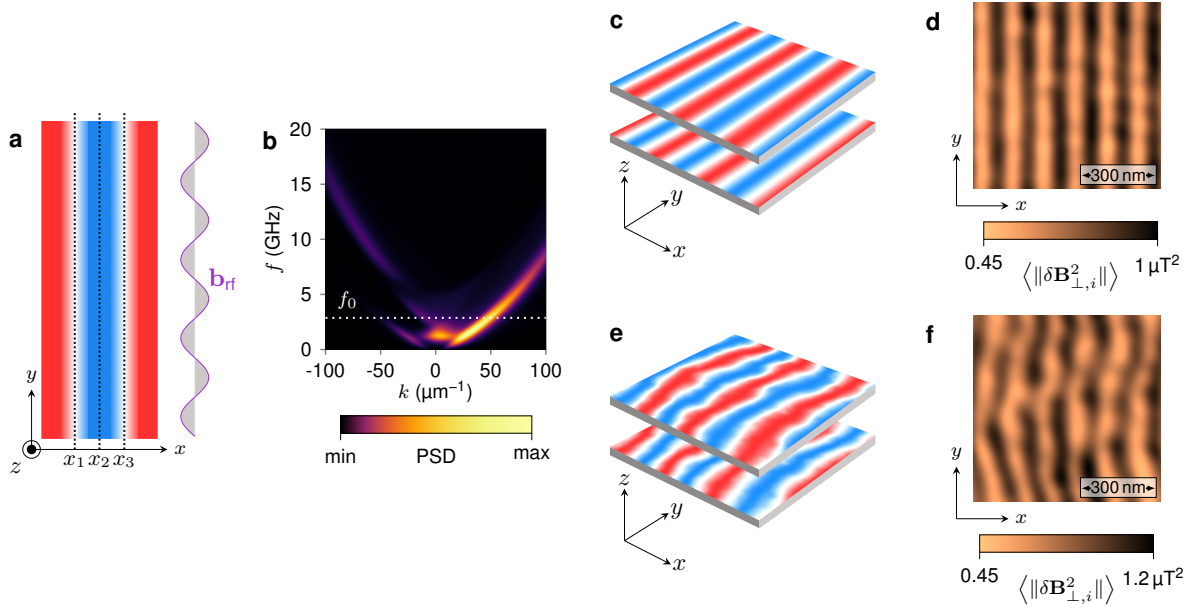

FIG. S3. **Spin wave dispersion relations and noise maps in SAF spin spirals.** **a**, Relaxed spin spiral configuration used for the calculation of the dispersion relation. The vertical dashed lines indicate the positions ( $x = x_1, x_2, x_3$ ) at which the spin wave response is computed, and  $b_{rf}$  denotes a schematic of the spatial sinusoidal field applied. **b**, Combined dispersion relations obtained at  $x = x_1, x_2, x_3$  in the geometry given in (b), where the dashed line indicates the NV frequency,  $f_0 = 2.87$  GHz. **c**, Relaxed spin spiral configuration used for magnetic noise intensity simulations. **d**, Simulated magnon noise map at  $f_0 = 2.87$  GHz for the configuration in **d** at 80 nm from the surface. **e**, Relaxed spin spiral configuration in the presence of magnetic disorder. **f**, Simulated magnon noise map at  $f_0$  for the configuration in **e** at 80 nm from the surface.

To compute the spin wave dispersion relations in the spin spiral, we follow the method used for the domain wall (Fig. 4c in the main text). We consider the transient response of the configuration in Figure S3a to a spatial sinusoidal field of different wave vectors, which are quantised by the length of the simulated geometry, with a sinc time dependence as discussed previously. The response is recorded at three positions along  $x$ : at the two channels along which  $m_z = 0$  (at  $x = x_1$  and  $x = x_3$  in Figure S3a) and at  $m_z = \pm 1$  (at  $x = x_2$  in Figure S3a). Because of the proximity of these three positions in the spin spiral, there is some intermixing between the modes and no clear distinction between “bulk” and

“channelled” as in the domain wall case. The simulated dispersion relations are shown in Figure S3b.

In Figure S3c, we show the relaxed spin spiral configuration for the calculation of the noise map. The geometry simulated is  $750 \times 750 \times 4.5 \text{ nm}^3$  in size that is discretized with  $512 \times 512 \times 3$  finite difference cells. The simulated noise map at 2.87 GHz is shown in Figure S3d, where we can observe a clear spatial contrast corresponding to the spin spiral configuration. The relaxed configuration in the presence of magnetic disorder is given in Figure S3e, where we can observe a roughening of the spirals. The corresponding noise map of the disordered system is presented in Figure S3f. Again, a clear contrast of the spin spiral can be observed which is strongly correlated with the shape of the equilibrium magnetic profile.

### C. Simulated noise spectrum of an isolated SAF skyrmion

To simulate the noise spectrum of an isolated SAF skyrmion, we used the same micromagnetic parameters as those for the spin spiral configuration with an additional static bias magnetic field,  $\mu_0 H_b = 50 \text{ mT}$ , which is applied to the bottom layer of the SAF. Since the effective perpendicular magnetic anisotropy is vanishing in this case, the presence of this bias field helps to stabilise the perpendicular magnetization. In Figure S4a, we plot the dispersion relation of the propagating spin waves in the uniform state with these parameters. These curves were obtained by linearizing the Landau-Lifshitz equation for the coupled dynamics of the top and bottom layer, using thin film approximations for the dipolar interactions [6]. In contrast to the case shown in Fig. 4b of the main text, where the spin wave gap scales with the perpendicular magnetic anisotropy, here the gap is largely dominated by the bias field applied to the bottom layer of the SAF, in conjunction with the interlayer exchange coupling, which also results in a larger frequency splitting between the two branches. The lower frequency branch, ‘t’, involves a stronger mode localization to the top magnetic layer in which the bias field is absent, while the higher frequency branch, ‘b’, involves stronger mode localization to the bottom magnetic layer in which the bias field is present. Another key difference compared with the spin wave spectrum in the uniform domains in Fig. 4 is the presence of excitation modes at the NV frequency. The inclusion of Gilbert damping results in the smeared PSD in Figure S4b, which shows a colour map computed from micromagnetics simulations.

The static magnetization profiles of the skyrmion in the top and bottom layers are shown in Figure S4c. The geometry simulated is  $750 \times 750 \times 4.5 \text{ nm}^3$  in size that is discretized with  $512 \times 512 \times 3$  finite difference cells. The simulated noise intensity map is shown in Figure S4d. Like for the domain wall and spin spiral cases, this map represents an average over 500 realisations of a random field with a harmonic time dependence at a frequency of 2.87 GHz. The map represents the values of the noise taken at 80 nm above the skyrmion. Despite the fact that the internal breathing mode frequencies of the skyrmion is above 2.87 GHz, we can observe a strong noise contrast at this frequency. We attribute this to the scattering of propagating spin waves with the skyrmion, which results in small displacements and deformations of the equilibrium profile. When disorder is included, we obtain the deformed skyrmion core as shown in the equilibrium profile in Figure S4e. The simulated noise map in Figure S4f reveals a smeared out contrast, both in the proximity of the skyrmion and within the domain, which arises from random scattering of the propagating spin waves at the NV frequency.

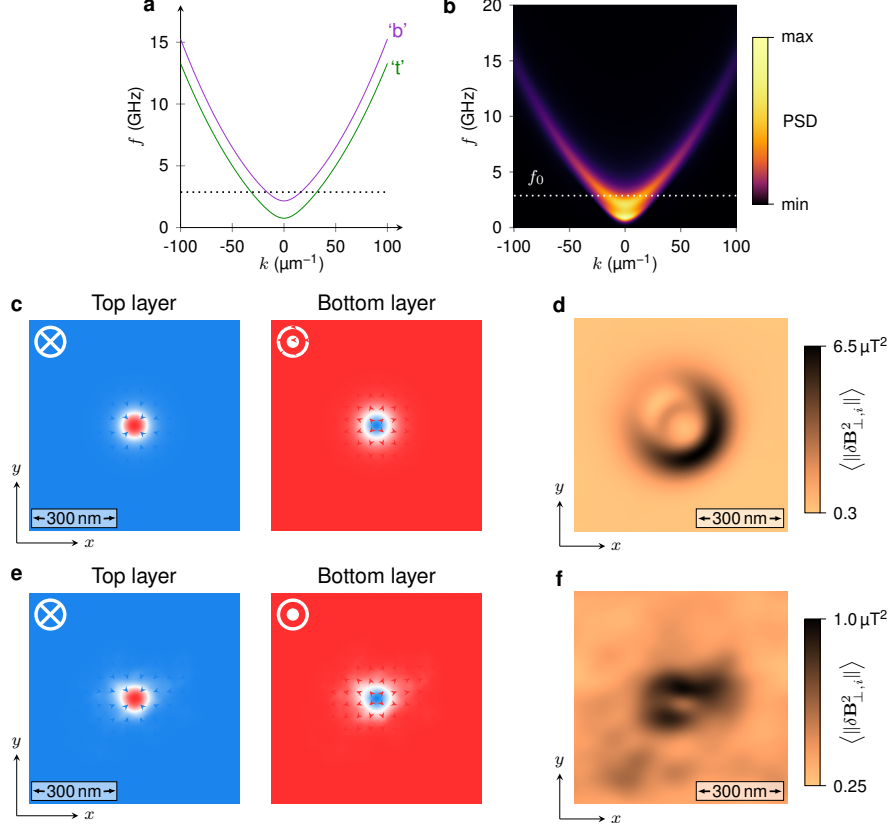

FIG. S4. **Noise spectrum of an isolated SAF skyrmion.** **a**, Theoretical dispersion relation for the uniform SAF domain with biasing on the bottom layer. ‘b’ and ‘t’ denote strong mode localization in the bottom and top layers of the SAF, respectively. **b**, Simulated dispersion relation for the domain state with  $\alpha = 0.1$ . The dashed lines in **a** and **b** indicate the NV frequency,  $f_0 = 2.87$  GHz. **c**, Relaxed magnetic configuration of the skyrmion. **d**, Simulated map of the magnetic noise intensity at  $f_0$  for the configuration in **c** at 80 nm from the surface. **e**, Relaxed magnetic configuration of the skyrmion in the presence of magnetic disorder. **f**, Simulated map of the magnetic noise intensity at  $f_0$  for the configuration in **e** at 80 nm from the surface.

#### D. Thermal power spectral density of the SAF uniform resonance mode

In the uniform state and in the absence of applied magnetic fields, the spin wave gap is determined by the anisotropy constant and interlayer exchange coupling, and corresponds to the precession frequency of the uniform resonance mode of the antiferromagnetically-coupled bilayer. While this gap is well above the NV frequency of 2.87 GHz at zero temperature, the presence of a large Gilbert damping constant of  $\alpha = 0.1$  results in a broadening of the spectral line such that the tail of the resonance peak overlaps the frequency range in which the NV spin relaxation is important. An example of the power spectrum is shown in Fig. S5, where the spectral line at  $T = 0$  K was computed from the Fourier transform of the transient response of  $\mathbf{m}_+(t) = \mathbf{m}_1(t) + \mathbf{m}_2(t)$  to the pulsed fields used to construct Fig. 4b of the main text. Indeed, this PSD represents the  $k = 0$  point in Fig. 4b.

To examine how this PSD evolves with temperature, we performed additional micromagnetics simulations with the MuMax3 code [3] that incorporate thermal effects through the

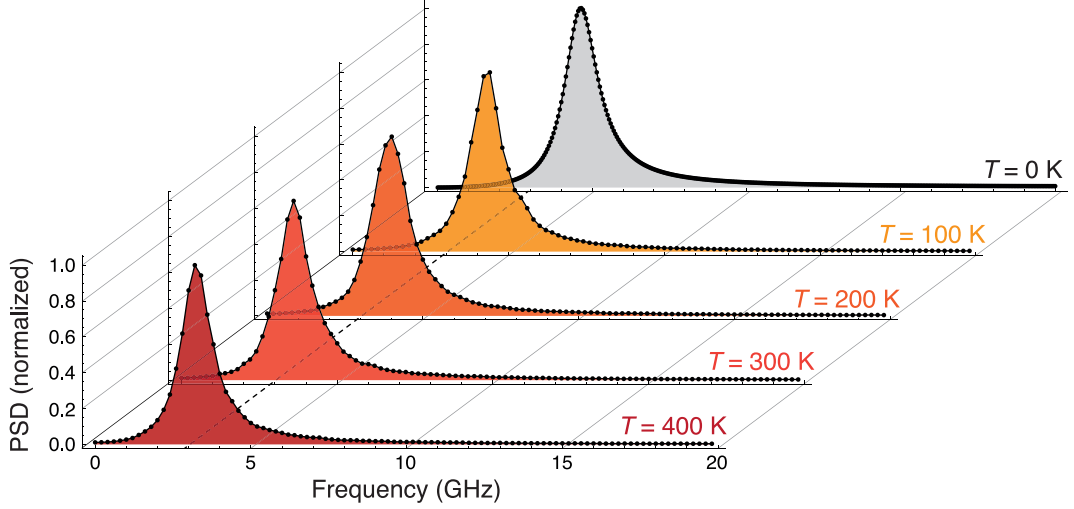

FIG. S5. **Thermal power spectral density (PSD) of the SAF uniform resonance mode.** At  $T = 0$  K, the PSD was computed from the transient response to a sinc field. At finite temperatures, the PSD was computed from the stochastic magnetization dynamics over  $2\mu\text{s}$ . The dashed line indicates the NV frequency of 2.87 GHz.

inclusion of a random thermal field [7–9]. For each value of the temperature considered, we perform the time integration of the stochastic dynamics over an interval of  $2\mu\text{s}$ . The power spectrum of  $\mathbf{m}_+(t)$  is then obtained by using the Welch method, which involves averaging over the spectra generated from the Fourier transform of half-overlapping 5-ns windows into which the original time series data is sliced. The thermal spectra are shown in Figure S5 for several values of the temperature. We observe that the uniform resonance frequency exhibits a noticeable downward frequency shift, from 4.6 GHz at  $T = 0$  K to 3.6 GHz at  $T = 300$  K. As such, it is likely that the relaxation broadening of this peak contributes to the observable reduction in  $T_1$  over uniform domains.

## IV. ADDITIONAL EXPERIMENTAL DATA

### A. Quantitative analysis of the domain wall profile

We compare the stray field profile of the domain wall presented in Figure 2 of the main text and again in Fig. S6a with the profile expected from micromagnetic simulations. The first step is to calibrate the distance  $d_{\text{NV}}$  between the NV sample and the surface. This is done using a well-characterized ferromagnetic stripe and by fitting the measured stray field profile produced at its edges, as detailed in ref. [10]. We obtain a value of  $d_{\text{NV}} = 80 \pm 5$  nm. In addition, the NV defect quantization axis was measured by recording the ESR frequency as a function of the amplitude and orientation of a calibrated magnetic field, leading to spherical angles  $\theta_{\text{NV}} = 58^\circ$  and  $\phi_{\text{NV}} = 103^\circ$ .

The magnetization profile of the domain wall plotted in Figure S6b-c is obtained from micromagnetic simulations with the parameters given in section III. Because of the dipolar coupling between the two layers, the wall width is larger in the top layer ( $w_{\text{top}} = 24$  nm) than in the bottom layer ( $w_{\text{bottom}} = 19.1$  nm). The stray field which is probed by the NV center above the surface of the SAF results from this width difference and from the vertical spacing between the two layers. As shown in Figure S6d, we computed the projection of the stray field along the NV axis, which is the sum of the contributions of each layer. The solid line is the profile at 80 nm from the surface and the colored area corresponds to a variation of  $\pm 5$  nm. The width of the measured peak is thinner than calculated, but this can be explained by drift during the scan because the domain wall is parallel to the fast scanning direction. We obtain a qualitative agreement with the experimental data in terms of field amplitude.

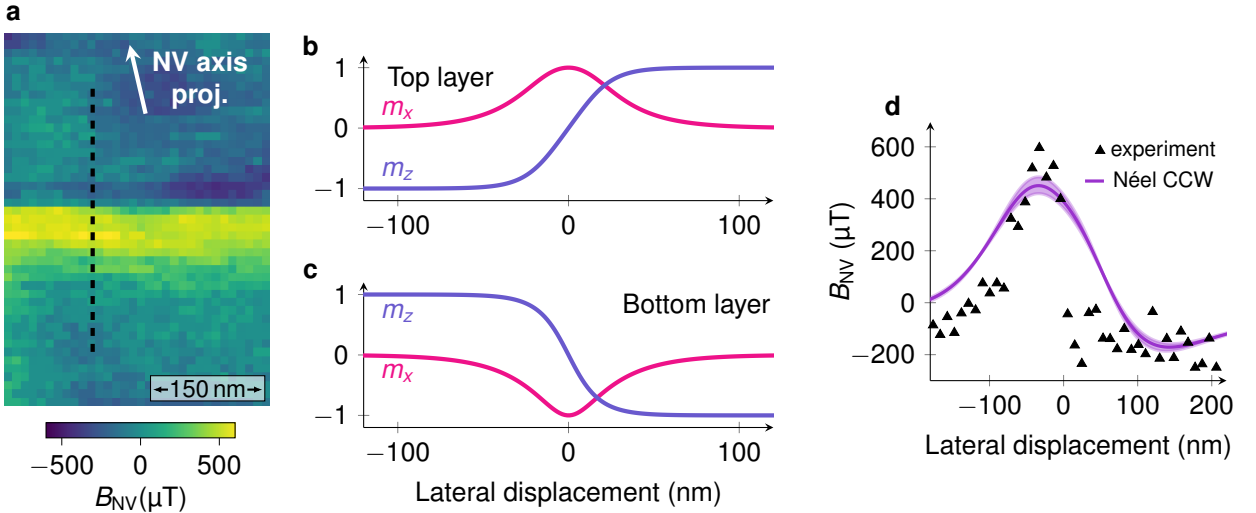

FIG. S6. **Analysis of the domain wall profile.** **a**, Field map recorded above a domain wall in a SAF sample, showing the component of the stray field oriented along the NV axis. **b**-, **c**, Magnetization profiles in the top (**b**) and bottom (**c**) layers from micromagnetic simulation. **d** Comparison between the experimental field profile and simulations of the expected stray field for a Néel wall with a counterclockwise rotational sense.

## B. Measurements of $T_1$ above non-magnetic surfaces

In order to check that the shortening of the  $T_1$  time observed when the NV center is placed above a magnetic domain has a magnetic origin (Fig. 3e), we performed similar experiments on non-magnetic samples. Figure S7a shows a relaxation curve with the tip far away from any surface, whereas the plots b and c display curves measured with the tip engaged on a Pt film or on a bulk diamond surface.

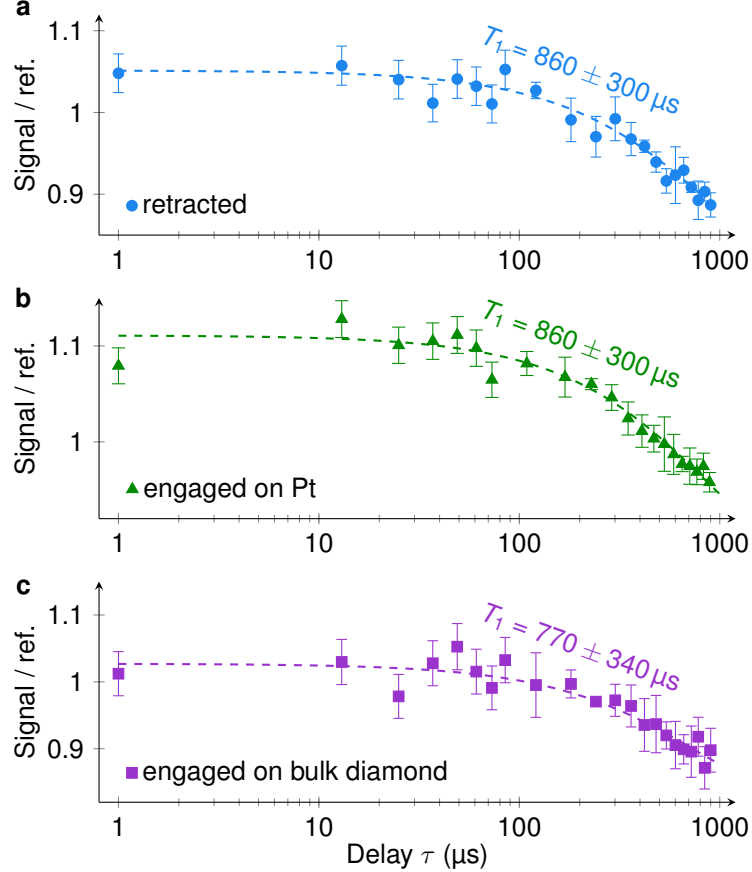

FIG. S7. **Relaxation time above non-magnetic surfaces.**  $T_1$  measurements comparing the situations with **a** the tip retracted and **b** engaged on a Pt film or **c** bulk diamond.

We do not observe any significant variations of  $T_1$  between these three cases. If the enhancement of the spin relaxation rate observed above a SAF domain was related to Johnson noise from the Pt capping layer of our magnetic samples, we should see a clear decrease of  $T_1$  when we approach the tip to a pure Pt layer. Our control experiments allow us to exclude this hypothesis. Shortening of  $T_1$  could also originate from charge state conversion of the NV center when it is brought very close to a surface, but again, if it was the case this should also occur during our control experiments. These measurements therefore indicate that the decrease of  $T_1$  measured when the tip is engaged on a SAF domain results from the presence of thermal population of magnons. This interpretation is further confirmed by the dispersion relation displayed in Fig. 4c of the main text and by the discussion about the effect of finite temperature in section IIID.

### C. Additional relaxation time measurements on the spin spiral sample

We performed measurements of the NV spin relaxation curve on the sample hosting the spin spiral, above the bright and the dark PL areas, as shown in Figure S8.  $T_1$  is smaller above the dark PL areas ( $T_1 = 400 \pm 40$  ns) than above the bright PL areas ( $T_1 = 920 \pm 60$  ns). The obtained values are much shorter than the one obtained on the sample hosting isolated domain walls. This is expected from the dispersion relation presented in Fig. S3b, with a very small gap and strong modes at  $f_0 = 2.87$  GHz. The detectable magnetic noise which they produce is more intense than in the domain wall sample.

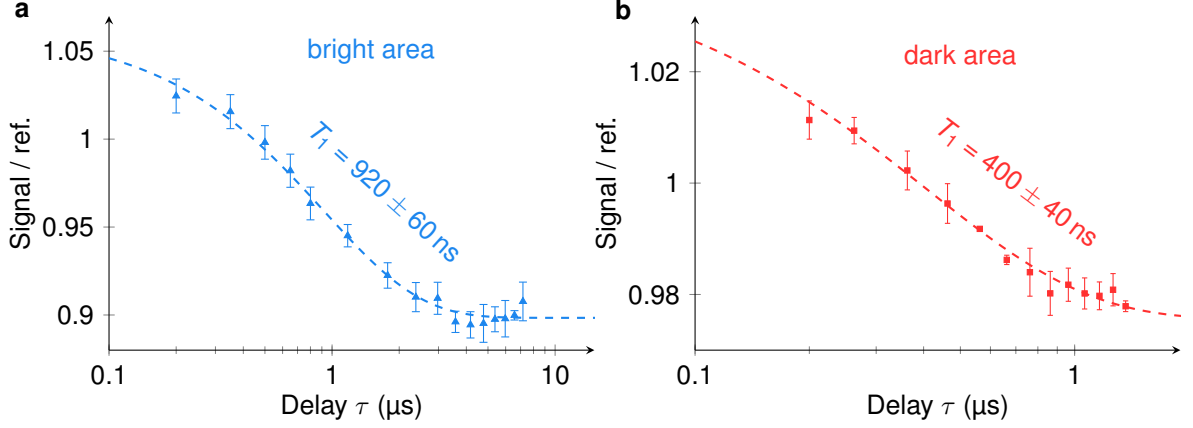

FIG. S8.  $T_1$  measurements on the spiral sample. NV spin relaxation curves measured above **a** the bright and **b** the dark PL areas of the spiral. We observe a reduction of  $T_1$  from  $920 \pm 60$  ns to  $400 \pm 40$  ns.

#### D. Additional relaxation time measurements on the skyrmion sample

We also measured  $T_1$  on the skyrmion sample (Figure S9). We obtain a decrease of  $T_1$  from  $9.1 \pm 0.6 \mu\text{s}$  above the background to  $870 \pm 60 \text{ ns}$  above the skyrmion. The  $T_1$  values are again very small, which can be explained by the dispersion shown in Fig S4. In this sample, the spin wave gap is much smaller than in the domain wall sample and strong modes are located in the NV detection zone in terms of frequency and wavelength.

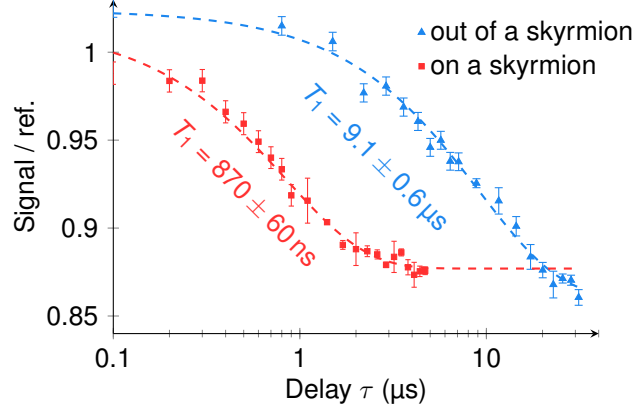

FIG. S9.  $T_1$  measurements on the skyrmion sample. NV spin relaxation curves measured above the background (blue triangles) and above a skyrmion (red squares). We observe a reduction of  $T_1$  when we place the tip above the skyrmion ( $T_1 = 870 \pm 60 \text{ ns}$ ) compared the value obtained far from the skyrmion ( $T_1 = 9.1 \pm 0.6 \mu\text{s}$ ).

- 
- [1] M. T. Johnson, P. J. H. Bloemen, F. J. A. d. Broeder, and J. J. d. Vries, *Reports on Progress in Physics* **59**, 1409 (1996).
  - [2] A. Dréau, M. Lesik, L. Rondin, P. Spinicelli, O. Arcizet, J.-F. Roch, and V. Jacques, *Physical Review B* **84**, 195204 (2011).
  - [3] A. Vansteenkiste, J. Leliaert, M. Dvornik, M. Helsen, F. Garcia-Sanchez, and B. Van Waeyenberge, *AIP Advances* **4**, 107133 (2014).
  - [4] J. Leliaert, B. Van de Wiele, A. Vansteenkiste, L. Laurson, G. Durin, L. Dupré, and B. Van Waeyenberge, *Journal of Applied Physics* **115**, 233903 (2014).
  - [5] C. L. Degen, F. Reinhard, and P. Cappellaro, *Reviews of Modern Physics* **89**, 035002 (2017).
  - [6] F. Nörtemann, R. L. Stamps, and R. E. Camley, *Physical Review B* **47**, 11910 (1993).
  - [7] W. Brown, *Physical Review* **130**, 1677 (1963).
  - [8] J. García-Palacios and F. Lázaro, *Physical Review B* **58**, 14937 (1998).
  - [9] J. Leliaert, J. Mulkers, J. De Clercq, A. Coene, M. Dvornik, and B. Van Waeyenberge, *AIP Advances* **7**, 125010 (2017).
  - [10] J.-P. Tetienne, T. Hingant, L. J. Martínez, S. Rohart, A. Thiaville, L. H. Diez, K. Garcia, J.-P. Adam, J.-V. Kim, J.-F. Roch, I. M. Miron, G. Gaudin, L. Vila, B. Ocker, D. Ravelosona, and V. Jacques, *Nature Communications* **6**, 6733 (2015).
